# Supplementary material for: Automated extraction of mutual independence patterns using Bayesian comparison of partition models
Source: arXiv:2001.05407 ancillary file (2020-01-15)
Supplement: Supplementary file 1 [file OnlineSupplement.pdf]

# Online supplement for manuscript "Automated extraction of mutual independence patterns using Bayesian comparison of partition models"

Guillaume Marrelec and Alain Giron

## Contents

**1 Results for the multivariate normal distribution 1**
1.1 Maximum likelihood . . . . . . . . . . . . . . . . . . . . . . . . 1
1.2 Bayesian inference with unknown mean and covariance . . . . 2
1.2.1 Marginal model likelihood . . . . . . . . . . . . . . . . . 2
1.2.2 Posterior probability . . . . . . . . . . . . . . . . . . . . 4

**2 Results for the cross-classified multinomial distribution 4**
2.1 Marginal model likelihood . . . . . . . . . . . . . . . . . . . . . 4
2.2 Asymptotic approximation . . . . . . . . . . . . . . . . . . . . . 5

**3 Results regarding partitions 6**
3.1 Asymptotic approximation for Bell numbers . . . . . . . . . . 6
3.2 Partitioning a set in two blocs . . . . . . . . . . . . . . . . . . . 7
3.3 Patterns of mutual independence and exchangeability . . . . 7
3.4 Patterns of mutual independence and consistency . . . . . . . 7

**4 Simulation study 9**
4.1 Gaussian data . . . . . . . . . . . . . . . . . . . . . . . . . . . . 9
4.2 Non-Gaussian data . . . . . . . . . . . . . . . . . . . . . . . . . 10

**5 HIV study data 14**

# 1 Results for the multivariate normal distribution

## 1.1 Maximum likelihood

Under the assumption of a partitioning into $K$ independent components, the likelihood reads

$$\mathrm{p}(\boldsymbol{S}|\mathcal{B},\boldsymbol{\Sigma}_1,\ldots,\boldsymbol{\Sigma}_K) = \frac{|\boldsymbol{S}|^{\frac{N-D-1}{2}}}{Z(D,N)} \prod_{k=1}^{K} |\boldsymbol{\Sigma}_k|^{-\frac{N}{2}} \exp\left[-\frac{1}{2}\mathrm{tr}\left(\boldsymbol{S}_k\boldsymbol{\Sigma}_k^{-1}\right)\right], \quad (1)$$

leading to a log-likelihood that is equal to

$$l(\boldsymbol{\Sigma}_1,\ldots,\boldsymbol{\Sigma}_K) = \mathrm{cst} - \sum_{k=1}^{K} \frac{N}{2}\left[\ln|\boldsymbol{\Sigma}_k| - \frac{1}{2}\mathrm{tr}\left(\boldsymbol{S}_k\boldsymbol{\Sigma}_k^{-1}\right)\right]. \tag{2}$$

It is the sum of $K$ independent terms, each of which is maximal for $\widehat{\boldsymbol{\Sigma}}_k = \boldsymbol{S}_k/N$ [1, Th. 3.2.1]. The corresponding maximum of the log-likelihood is

$$l(\widehat{\boldsymbol{\Sigma}}_1,\ldots,\widehat{\boldsymbol{\Sigma}}_K) = \mathrm{cst} - \sum_{k=1}^{K} \frac{N}{2}\ln|\widehat{\boldsymbol{\Sigma}}_k| - \frac{ND}{2}. \tag{3}$$

The only part of this expression that *does* depend on the partitioning induced by $\mathcal{B}$ is

$$-\sum_{k=1}^{K} \frac{N}{2}\ln|\widehat{\boldsymbol{\Sigma}}_k|. \tag{4}$$

## 1.2 Bayesian inference with unknown mean and covariance

### 1.2.1 Marginal model likelihood

**Case of one vector.** Computation of the marginal model likelihood for the full dataset and i.i.d. multivariate normal distribution yields

$$\begin{aligned}\mathrm{p}(\boldsymbol{x}|\mathcal{B}) &= \int \mathrm{p}(\boldsymbol{x},\boldsymbol{\mu},\boldsymbol{\Sigma}|\mathcal{B})\,\mathrm{d}\boldsymbol{\mu}\,\mathrm{d}\boldsymbol{\Sigma}\\ &= \int \mathrm{p}(\boldsymbol{x}|\mathcal{B},\boldsymbol{\mu},\boldsymbol{\Sigma})\,\mathrm{p}(\boldsymbol{\mu},\boldsymbol{\Sigma}|\mathcal{B})\,\mathrm{d}\boldsymbol{\mu}\mathrm{d}\,\boldsymbol{\Sigma}.\end{aligned} \tag{5}$$

The likelihood for the whole dataset reads

$$\mathrm{p}(\boldsymbol{\mu},\boldsymbol{\Sigma}|\mathcal{B}) = (2\pi)^{-\frac{ND}{2}}|\boldsymbol{\Sigma}|^{-\frac{N}{2}}\exp\left[-\frac{1}{2}\sum_n(\boldsymbol{x}_n-\boldsymbol{\mu})^{\mathrm{t}}\boldsymbol{\Sigma}^{-1}(\boldsymbol{x}_n-\boldsymbol{\mu})\right]. \tag{6}$$

Following [2, §3.6], we set conjugate priors for $\boldsymbol{\Sigma}$ and $\boldsymbol{\mu}$: Inverse-Wishart with $\nu$ degrees of freedom and inverse scale matrix $\boldsymbol{\Lambda}$ for $\boldsymbol{\Sigma}$; multivariate normal with mean $\boldsymbol{\lambda}$ and covariance matrix $\boldsymbol{\Sigma}/\kappa$ for $\boldsymbol{\mu}$:

$$\mathrm{p}(\boldsymbol{\Sigma}|\mathcal{B}) = \frac{|\boldsymbol{\Lambda}|^{\frac{\nu}{2}}}{Z(D,\nu)}|\boldsymbol{\Sigma}|^{-\frac{\nu+D+1}{2}}\exp\left[-\frac{1}{2}\mathrm{tr}(\boldsymbol{\Sigma}^{-1}\boldsymbol{\Lambda})\right] \tag{7}$$

$$\mathrm{p}(\boldsymbol{\mu}|\mathcal{B},\boldsymbol{\Sigma}) = (2\pi)^{-\frac{D}{2}}\left|\frac{\boldsymbol{\Sigma}}{\kappa}\right|^{-\frac{1}{2}}\exp\left[-\frac{1}{2}(\boldsymbol{\mu}-\boldsymbol{\lambda})^{\mathrm{t}}\left(\frac{\boldsymbol{\Sigma}}{\kappa}\right)^{-1}(\boldsymbol{\mu}-\boldsymbol{\lambda})\right]. \tag{8}$$

The product $\mathrm{p}(\boldsymbol{x}|\mathcal{B},\boldsymbol{\mu},\boldsymbol{\Sigma})\,\mathrm{p}(\boldsymbol{\mu},\boldsymbol{\Sigma}|\mathcal{B})$ can therefore be expressed as

$$\begin{aligned}&(2\pi)^{-\frac{D(N+1)}{2}}|\boldsymbol{\Sigma}|^{-\frac{N+\nu+D+2}{2}}\kappa^{\frac{D}{2}}\frac{|\boldsymbol{\Lambda}|^{\frac{\nu}{2}}}{Z(D,\nu)}\\ &\times\exp\left\{-\frac{1}{2}\left[(N+\kappa)(\boldsymbol{\mu}-\widehat{\boldsymbol{\mu}})^{\mathrm{t}}\boldsymbol{\Sigma}^{-1}(\boldsymbol{\mu}-\widehat{\boldsymbol{\mu}}) + \mathrm{tr}\left\{\boldsymbol{\Sigma}^{-1}\left[\boldsymbol{S}+\boldsymbol{\Lambda}+\frac{N\kappa}{N+\kappa}(\boldsymbol{m}-\boldsymbol{\lambda})(\boldsymbol{m}-\boldsymbol{\lambda})^{\mathrm{t}}\right]\right\}\right]\right\},\end{aligned} \tag{9}$$

where $\boldsymbol{m}$ is the sample mean. As a function of $\boldsymbol{\mu}$, this quantity is proportional to a multivariate normal distribution with mean $\widehat{\boldsymbol{\mu}}$ and covariance matrix $\boldsymbol{\Sigma}/(N+\kappa)$. Integration with respect to $\boldsymbol{\mu}$ therefore involves multiplication by

$$(2\pi)^{\frac{D}{2}} \left| \frac{\boldsymbol{\Sigma}}{N+\kappa} \right|^{\frac{1}{2}}, \tag{10}$$

yielding

$$\begin{aligned} &(2\pi)^{-\frac{DN}{2}} |\boldsymbol{\Sigma}|^{-\frac{N+\nu+D+1}{2}} \left(\frac{\kappa}{N+\kappa}\right)^{\frac{D}{2}} \frac{|\boldsymbol{\Lambda}|^{\frac{\nu}{2}}}{Z(D,\nu)} \\ &\quad \times \exp\left(-\frac{1}{2}\mathrm{tr}\left\{\boldsymbol{\Sigma}^{-1}\left[\boldsymbol{S}+\boldsymbol{\Lambda}+\frac{N\kappa}{N+\kappa}(\boldsymbol{m}-\boldsymbol{\lambda})(\boldsymbol{m}-\boldsymbol{\lambda})^{\mathsf{t}}\right]\right\}\right). \end{aligned} \tag{11}$$

As a function of $\boldsymbol{\Sigma}$, this quantity is proportional to an inverse-Wishart distribution with $N+\nu$ degrees of freedom and inverse scale matrix

$$\boldsymbol{S}+\boldsymbol{\Lambda}+\frac{N\kappa}{N+\kappa}(\boldsymbol{m}-\boldsymbol{\lambda})(\boldsymbol{m}-\boldsymbol{\lambda})^{\mathsf{t}}. \tag{12}$$

Integration with respect to $\boldsymbol{\Sigma}$ therefore involves multiplication by

$$Z(D,N+\nu) \left| \boldsymbol{S}+\boldsymbol{\Lambda}+\frac{N\kappa}{N+\kappa}(\boldsymbol{m}-\boldsymbol{\lambda})(\boldsymbol{m}-\boldsymbol{\lambda})^{\mathsf{t}} \right|^{-\frac{N+\nu}{2}}, \tag{13}$$

finally yielding

$$\mathrm{p}(\boldsymbol{x}|\mathcal{B}) = (2\pi)^{-\frac{DN}{2}} \left(\frac{\kappa}{N+\kappa}\right)^{\frac{D}{2}} \frac{Z(D,N+\nu)}{Z(D,\nu)} \frac{|\boldsymbol{\Lambda}|^{\frac{\nu}{2}}}{\left|\boldsymbol{S}+\boldsymbol{\Lambda}+\frac{N\kappa}{N+\kappa}(\boldsymbol{m}-\boldsymbol{\lambda})(\boldsymbol{m}-\boldsymbol{\lambda})^{\mathsf{t}}\right|^{\frac{N+\nu}{2}}}. \tag{14}$$

**Case of several independent subvectors.** If we have several independent subvectors instead, a similar calculation can be performed, leading to

$$\begin{aligned} \mathrm{p}(\boldsymbol{x}|\mathcal{B}) &= (2\pi)^{-\frac{DN}{2}} \left(\frac{\kappa}{N+\kappa}\right)^{\frac{D}{2}} \\ &\quad \times \prod_{k=1}^{K} \frac{Z(D_k,N+\nu_k)}{Z(D_k,\nu_k)} \frac{|\boldsymbol{\Lambda}_k|^{\frac{\nu_k}{2}}}{\left|\boldsymbol{S}_k+\boldsymbol{\Lambda}_k+\frac{N\kappa}{N+\kappa}(\boldsymbol{m}_k-\boldsymbol{\lambda}_k)(\boldsymbol{m}_k-\boldsymbol{\lambda}_k)^{\mathsf{t}}\right|^{\frac{N+\nu_k}{2}}}. \end{aligned} \tag{15}$$

### 1.2.2 Posterior probability

The posterior distribution for a given model of dependence can then be obtained by application of Bayes' theorem, yielding

$$\Pr(\mathcal{B}|\boldsymbol{x}) \propto \Pr(\mathcal{B})\, \mathrm{p}(\boldsymbol{x}|\mathcal{B}). \tag{16}$$

Since

$$(2\pi)^{-\frac{DN}{2}} \left(\frac{\kappa}{N+\kappa}\right)^{\frac{D}{2}} \tag{17}$$

does not depend on $\mathcal{B}$, this quantity does not change when $h$ changes. It therefore disappears in the normalization constant and we have

$$\Pr(\mathcal{B}|\boldsymbol{x}) \quad \propto \quad \Pr(\mathcal{B}) \prod_{k=1}^{K} \frac{Z(D_k, N+\nu_k)}{Z(D_k, \nu_k)} \frac{|\boldsymbol{\Lambda}_k|^{\frac{\nu_k}{2}}}{\left|\boldsymbol{S}_k + \boldsymbol{\Lambda}_k + \frac{N\kappa}{N+\kappa}(\boldsymbol{m}_k - \boldsymbol{\lambda}_k)(\boldsymbol{m}_k - \boldsymbol{\lambda}_k)^{\mathrm{t}}\right|^{\frac{N+\nu_k}{2}}}. \tag{18}$$

Setting $\kappa \to 0$, we obtain the result of Equation (14).

# 2 Results for the cross-classified multinomial distribution

## 2.1 Marginal model likelihood

The marginalization formula yields

$$\Pr(\boldsymbol{y}|\mathcal{B}) = \int \mathrm{p}(\boldsymbol{\theta}_1, \ldots, \boldsymbol{\theta}_K)\ \Pr(\boldsymbol{y}|\boldsymbol{\theta}_1, \ldots, \boldsymbol{\theta}_K) \prod_{k=1}^{K} \mathrm{d}\boldsymbol{\theta}_k. \tag{19}$$

Assuming that the different parameters are a priori independent, the prior distribution reads

$$\mathrm{p}(\boldsymbol{\theta}_1, \ldots, \boldsymbol{\theta}_K) = \prod_{k=1}^{K} \mathrm{p}(\boldsymbol{\theta}_k), \tag{20}$$

where, for each $\mathrm{p}(\boldsymbol{\theta}_k)$, we set a Dirichlet distribution with parameters $a_{\boldsymbol{x}_k}$ for $\boldsymbol{x}_k \in E_{B_k}$

$$\mathrm{p}(\boldsymbol{\theta}_k) = \frac{\Gamma\left(\sum_{\boldsymbol{x}_k \in E_{B_k}} a_{\boldsymbol{x}_k}\right)}{\prod_{\boldsymbol{x}_k \in E_{B_k}} \Gamma(a_{\boldsymbol{x}_k})} \prod_{\boldsymbol{x}_k \in E_{B_k}} \theta_{\boldsymbol{x}_k}^{a_{\boldsymbol{x}_k}}. \tag{21}$$

According to the assumption of mutual independence, we have for the likelihood

$$\Pr(\boldsymbol{y}|\boldsymbol{\theta}_1, \ldots, \boldsymbol{\theta}_K) = \prod_{k=1}^{K} \Pr(\boldsymbol{y}_k|\boldsymbol{\theta}_k), \tag{22}$$

with

$$\Pr(\boldsymbol{y}_k|\boldsymbol{\theta}_k) = \prod_{\boldsymbol{x}_k \in E_{B_k}} \theta_{\boldsymbol{x}_k}^{N_{\boldsymbol{x}_k}}, \tag{23}$$

where $N_{\boldsymbol{x}_k}$ is the number of time that we observe $\boldsymbol{x}_k$. Putting the prior and likelihood together into Bayes' theorem yields for the marginal model likelihood

$$\Pr(\boldsymbol{y}|\mathcal{B}) = \prod_{k=1}^{K} \frac{\Gamma\left(\sum_{\boldsymbol{x}_k \in E_{B_k}} a_{\boldsymbol{x}_k}\right)}{\prod_{\boldsymbol{x}_k \in E_{B_k}} \Gamma(a_{\boldsymbol{x}_k})} \int \prod_{\boldsymbol{x}_k \in E_{B_k}} \theta_{\boldsymbol{x}_k}^{N_{\boldsymbol{x}_k}+a_{\boldsymbol{x}_k}} \, \mathrm{d}\boldsymbol{\theta}_k. \tag{24}$$

As a function of $\boldsymbol{\theta}_k$, this expression is proportional to a Dirichlet distribution with parameters $N_{\boldsymbol{x}_k} + a_{\boldsymbol{x}_k}$ for $\boldsymbol{x}_k \in E_{B_k}$. Integration with respect to $\boldsymbol{\theta}_k$ therefore yields

$$\Pr(\boldsymbol{y}|\mathcal{B}) = \prod_{k=1}^{K} \frac{\Gamma\left(\sum_{\boldsymbol{x}_k \in E_{B_k}} a_{\boldsymbol{x}_k}\right)}{\prod_{\boldsymbol{x}_k \in E_{B_k}} \Gamma(a_{\boldsymbol{x}_k})} \frac{\prod_{\boldsymbol{x}_k \in E_{B_k}} \Gamma(N_{\boldsymbol{x}_k} + a_{\boldsymbol{x}_k})}{\Gamma\left(\sum_{\boldsymbol{x}_k \in E_{B_k}} N_{\boldsymbol{x}_k} + a_{\boldsymbol{x}_k}\right)}. \tag{25}$$

## 2.2 Asymptotic approximation

From the previous equation, we have

$$\ln \Pr(\boldsymbol{y}|\mathcal{B}) = \sum_{k=1}^{K} \left[ \sum_{\boldsymbol{x}_k \in E_{B_k}} \ln \Gamma(N_{\boldsymbol{x}_k} + a_{\boldsymbol{x}_k}) - \ln \Gamma\left( \sum_{\boldsymbol{x}_k \in E_{B_k}} N_{\boldsymbol{x}_k} + a_{\boldsymbol{x}_k} \right) \right] + \text{cst}, \tag{26}$$

where "cst" is a term that does not depend on the data. Set

$$a_k = \sum_{\boldsymbol{x}_k \in E_{B_k}} a_{\boldsymbol{x}_k}$$

and $f_{\boldsymbol{x}_k} = N_{\boldsymbol{x}_k}/N$, so that $\sum_{\boldsymbol{x}_k \in E_{B_k}} f_{\boldsymbol{x}_k} = 1$. In the following, we assume large data set, $N \to \infty$ and use the following approximation for the Gamma function [3, p. 257]

$$\ln \Gamma(z) = \left(z - \frac{1}{2}\right) \ln z - z + O(1). \tag{27}$$

We have

$$\begin{aligned} \ln \Gamma(N + a_k) &= \left(N + a_k - \frac{1}{2}\right) \ln(N + a_k) - (N + a_k) + O(1) \\ &= N \ln N - N + \left(a_k - \frac{1}{2}\right) \ln N + O(1) \end{aligned} \tag{28}$$

and, similarly,

$$\begin{aligned}\ln\Gamma(N_{\boldsymbol{x}_k}+a_{\boldsymbol{x}_k}) &= \ln\Gamma(f_{\boldsymbol{x}_k}N+a_{\boldsymbol{x}_k})\\ &= \left(f_{\boldsymbol{x}_k}N+a_{\boldsymbol{x}_k}-\frac{1}{2}\right)\ln(f_{\boldsymbol{x}_k}N+a_{\boldsymbol{x}_k})-(f_{\boldsymbol{x}_k}N+a_{\boldsymbol{x}_k})+O(1)\\ &= f_{\boldsymbol{x}_k}N\ln N+N(f_{\boldsymbol{x}_k}\ln f_{\boldsymbol{x}_k}-f_{\boldsymbol{x}_k})+\left(a_{\boldsymbol{x}_k}-\frac{1}{2}\right)\ln N+O(1).\end{aligned} \tag{29}$$

Putting these two results together yields for the log marginal model likelihood

$$\ln\Pr(\boldsymbol{y}|\mathcal{B})=\sum_{k=1}^{K}\left[N\sum_{\boldsymbol{x}_k\in E_{B_k}}f_{\boldsymbol{x}_k}\ln f_{\boldsymbol{x}_k}-\frac{I_{B_k}-1}{2}\ln N\right]+O(1). \tag{30}$$

Considering the log posterior distribution instead of the marginal model likelihood only adds the log prior which is itself $O(1)$.

**Maximum-likelihood estimate.** For model $H$ and block $k$, the maximum-likelihood estimate is given by

$$\widehat{\theta}_{\boldsymbol{x}_k}=\frac{N_{\boldsymbol{x}_k}}{N}=f_{\boldsymbol{x}_k}. \tag{31}$$

The corresponding maximum of the log-likelihood is then equal to

$$\ln\Pr(\boldsymbol{y}|\widehat{\boldsymbol{\theta}}_1,\ldots,\widehat{\boldsymbol{\theta}}_K)=\sum_{k=1}^{K}N\sum_{\boldsymbol{x}_k\in E_{B_k}}f_{\boldsymbol{x}_k}\ln f_{\boldsymbol{x}_k}, \tag{32}$$

which corresponds to the the first term in the right-hand side of the above approximation.

# 3 Results regarding partitions

## 3.1 Asymptotic approximation for Bell numbers

We have the following asymptotic approximation [4, §6.2]

$$\frac{\ln\varpi_D}{D}=\ln D-\ln\ln D-1+O\left(\frac{\ln\ln D}{\ln D}\right), \tag{33}$$

showing that

$$\varpi_D=O\left[\left(\frac{D}{\ln D}\right)^D\right], \tag{34}$$

see also [5, §7.2.1.5].

### 3.2 Partitioning a set in two blocs

We here prove that $\left\{ {d \atop 2} \right\} = 2^{d-1} - 1$. First, there is a one-to-one mapping between the set of functions $\phi : [d] \to \{0,1\}^d$ and the set of partitioning of $[d]$ into two subsets $A$ and $B$ (for instance, by translating $\phi(i) = 0$ to $i \in A$ and $\phi(i) = 1$ to $i \in B$). There are $2^d$ such functions. Among these functions, two correspond to a partitioning of $[d]$ into only one block: $\phi([d]) = \{0\}^d$ (corresponding to $A = [d]$ and $B = \emptyset$) and $\phi([d]) = \{1\}^d$ (corresponding to $A = \emptyset$ and $B = [d]$), which we remove, leaving ony $2^d - 2$ functions. Finally, each function $\phi$ can be uniquely associated to a different function $\psi$ that only switches labels $A$ and $B$, for instance, by defining $\psi$ such that $\psi(i) = 1 - \phi(i)$. Since the labels do not interest us for partitioning, we are left with $(2^d - 2)/2 = 2^{d-1} - 1$ distinct cases.

### 3.3 Patterns of mutual independence and exchangeability

We here give a quick example of the implication of assuming exchangeability for the prior distribution on partitions. Consider the case of $D = 3$ variables $X_1$, $X_2$, and $X_3$. There are $\varpi_3 = 5$ potential partitions: $1|2|3$, $12|3$, $13|2$, $23|1$, and $123$. Since $13|2$ can be obtained from $12|3$ by permutation of labels 2 and 3, exchangeability requires for a prior $P_3$

$$P_3([12|3]) = P_3([13|2]). \tag{35}$$

Similarly, since $23|1$ can be obtained from $12|3$ by permutation of labels 1 and 3,

$$P_3([12|3]) = P_3([23|1]). \tag{36}$$

So, to define $P_3$, we would have to set $P_3([1|2|3])$, $P_3([12|3]) = P_3([13|2]) = P_3([23|1])$ and $P_3([123])$, with the further constraint that all probabilities sum to 1, i.e.,

$$P_3([1|2|3]) + 3P_3([12|3]) + P_3([123]) = 1. \tag{37}$$

### 3.4 Patterns of mutual independence and consistency

We here demonstrate why the requirement of having a prior distribution on the set of partitions that is consistent in the sense of [6] is not valid for patterns of mutual independence. Consistency relies on the fact that a prior can be generated constructively from a set with $D$ variables by adding one variable, leading to a set with $D + 1$ variables. In our case, it implies that knowing the pattern of mutual independence between $D$ variables strongly constrains the pattern of mutual independence of the same $D$ variables to which one extra variable is added. In the simple case $D = 2$, assuming consistency would imply that the pattern of mutual independence between $X_1$ and $X_2$ constrains that between $X_1$, $X_2$, and $X_3$. Unfortunately, this is not true.

Two variables $X_1$ and $X_2$ can potentially be partitioned in $\varpi_2 = 2$ different ways, namely the one-block partition 12 and the two-block partition 1|2. Adding one variable $X_3$, there are $\varpi_3 = 5$ potential partitions: 1|2|3, 12|3, 13|2, 23|1, and 123. Since adding 3 to partition 12 can be done in two different ways, namely 12|3 and 123, consistency would require[1]

$$P_2([12]) = P_3([12|3]) + P_3([123]). \tag{38}$$

Similarly, since adding 3 to partition 1|2 can be done in three different ways, namely 13|2, 1|23, and 1|2|3, consistency would entail

$$P_2([1|2]) = P_3([1|2|3]) + P_3([12|3]) + P_3([1|23]). \tag{39}$$

In words, this second case means that knowing that $X_1$ and $X_2$ are independent (i.e., the correct partition is 1|2) when considering only these two variables entails that the pattern of dependence between $X_1$, $X_2$, and $X_3$ has to be either 1|2|3, 12|3, or 1|23; in particular, it *cannot* be 123.

To show that this is not true, assume that $X_1$, $X_2$ and $X_3$ are related through the directed acyclic graph depicted in Figure 1. $X_1$ and $X_2$ are independent, corresponding to partition 1|2, yet we neither have $(X_1, X_3)$ and $X_2$ mutually independent (which would correspond to partition 13|2) nor $(X_2, X_3)$ and $X_1$ mutually independent (which would correspond to partition 1|23, nor $X_1$, $X_2$, and $X_3$ mutually independent (which would correspond to partition 1|2|3). The correct partition is 123. This is a consequence of the fact that, while the distribution of $(X_1, X_2, X_3)$ (from which we can determine the pattern of mutual independence between $X_1$, $X_2$, and $X_3$) makes it possible to determine the marginal of $(X_1, X_2)$ (from which we can determine the pattern of mutual independence between $X_1$ and $X_2$), the converse does not hold.

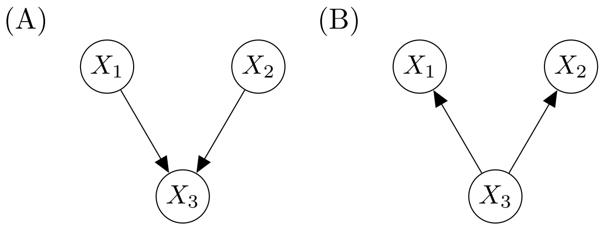


Figure 1: Mutual independence may not respect consistency. (A) Example where $X_1$ and $X_2$ are independent, corresponding to partition 1|2, yet there is no mutual independence between $X_1$, $X_2$ and $X_3$, corresponding to partition 123. (B) Example where $X_1$ and $X_2$ are not independent, corresponding to partition 12, and where there is again no mutual independence between $X_1$, $X_2$ and $X_3$, corresponding to partition 123.

[1] In the following, we put partition models that appear in probabilities between brackets, to make it clear that the "|" sign should *not* be interpreted as a conditioning sign.

# 4 Simulation study

## 4.1 Gaussian data

We plotted the relationship between `BayesOptim` and either `BayesCorr` (Fig. 2) or `Bic` (Fig. 3) depending on the number of clusters in the simulated Gaussian data.

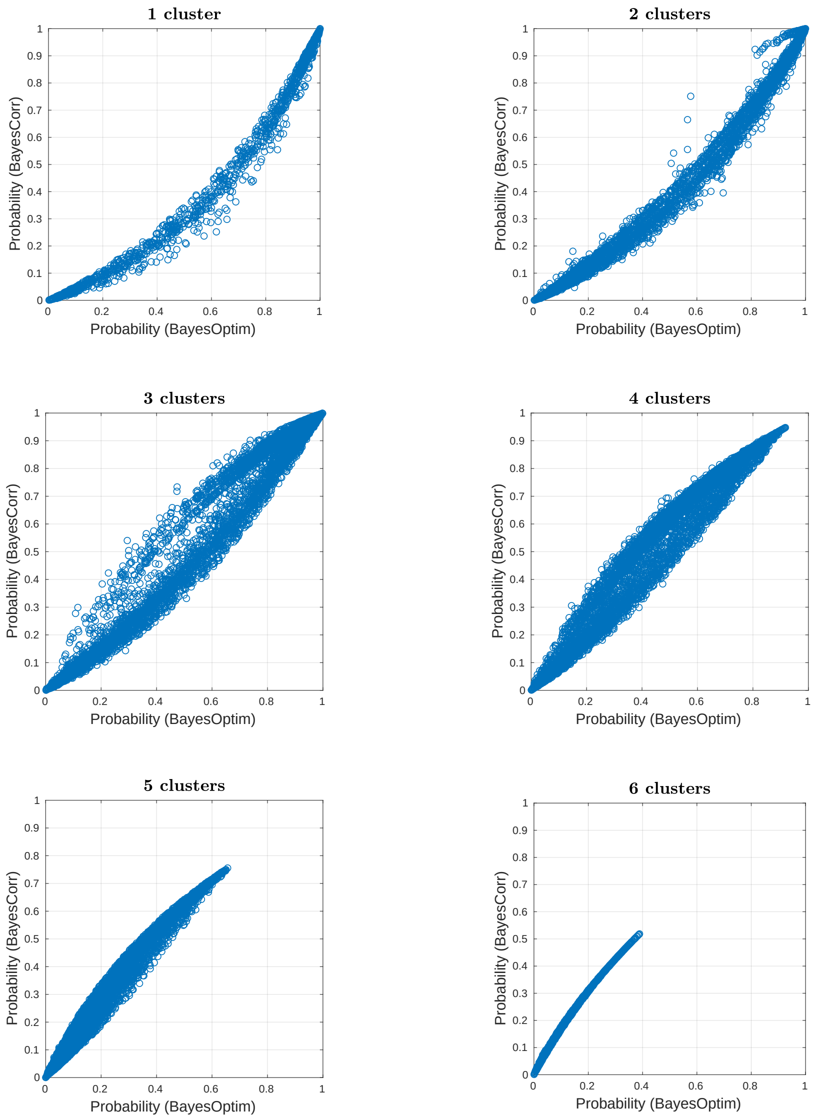


Figure 2: **Simulation study.** Comparison of probability obtained for `BayesOptim` and `BayesCorr` depending on the number of clusters in the simulated Gaussian data.

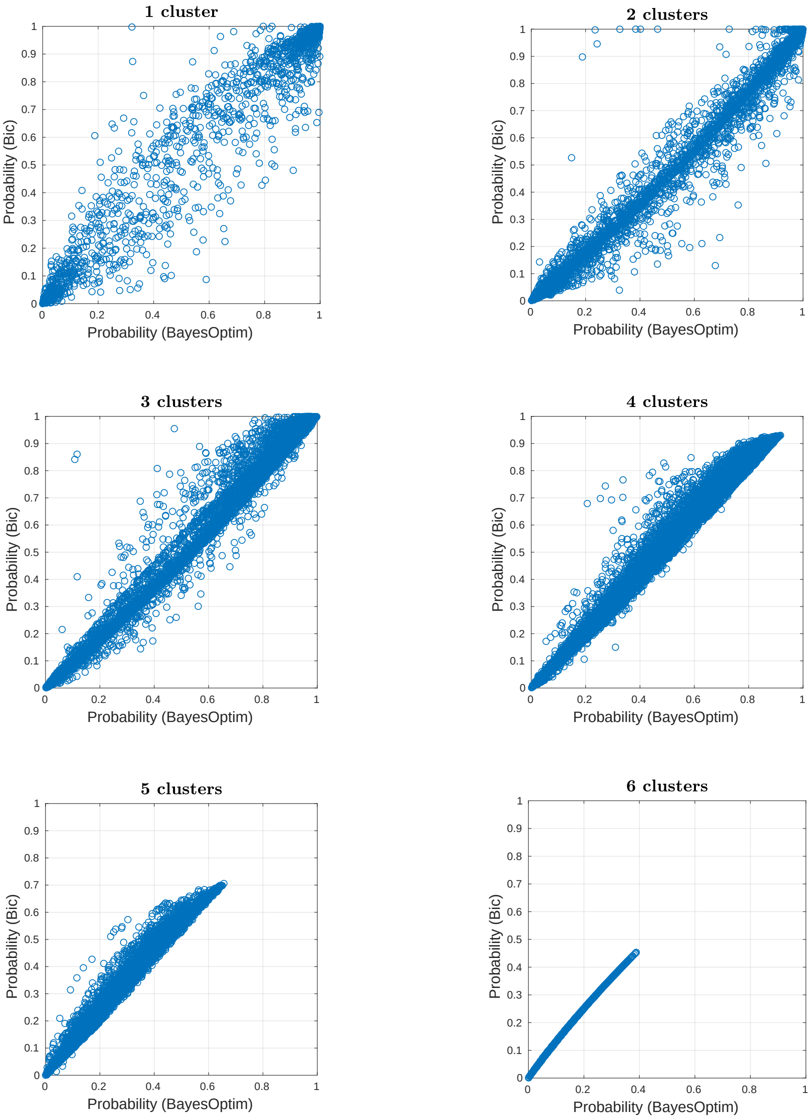


Figure 3: **Simulation study.** Comparison of probability obtained for `BayesOptim` and `Bic` depending on the number of clusters in the simulated Gaussian data.

## 4.2 Non-Gaussian data

We plotted the global relationship between `BayesOptim` and either `BayesCorr` or `Bic` depending on the degree of freedom of the Student-$t$ distributions and the number of clusters in the simulated non-Gaussian data (Fig. 4). For `BayesOptim`, we plotted the evolution of four quantities as a function of sample size: posterior probability of the true model, and ratio of posterior probability of true model to posterior probability of maximum a posteriori

(Fig. 5); rank of true model when ranking potential models by decreasing posterior probability, and entropy of posterior distribution (Fig. 6).

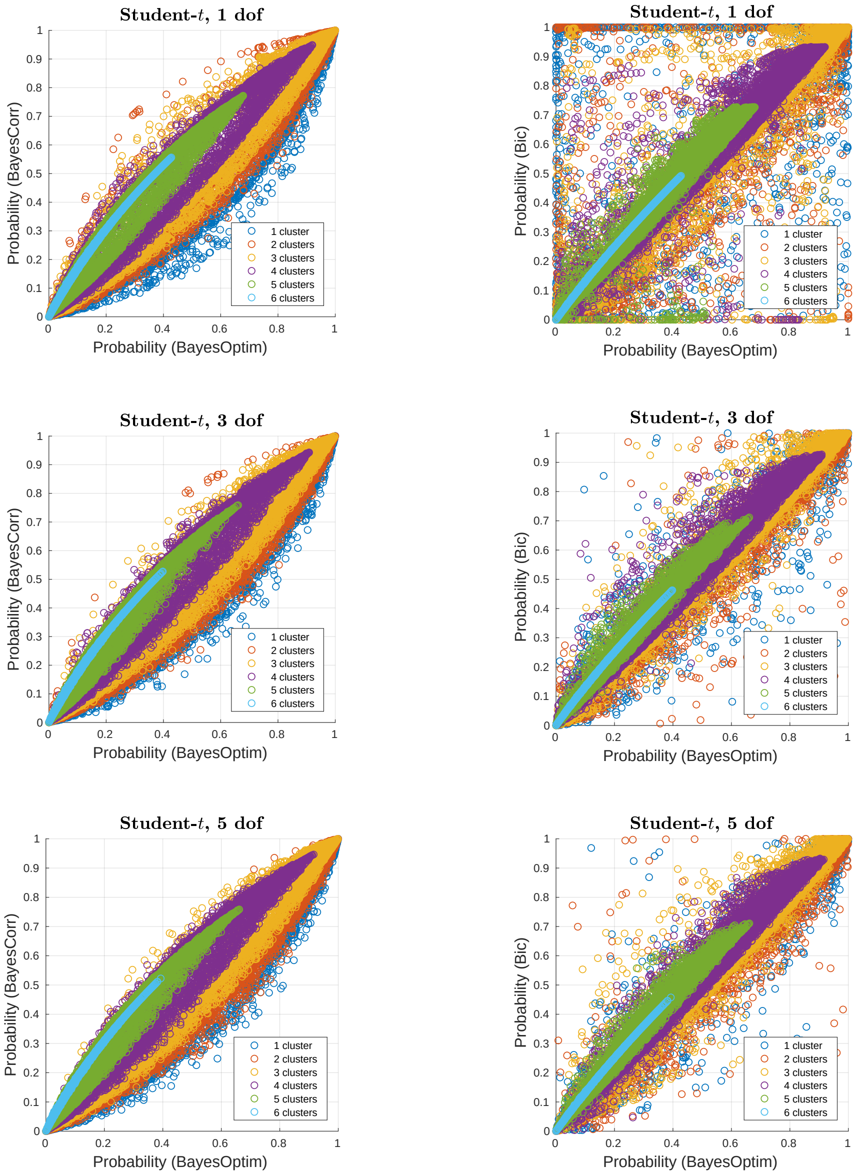


Figure 4: **Simulation study.** Comparison of probability obtained for `BayesOptim` and either `BayesCorr` (left) or `Bic` (right) depending on the number of degrees of freedom of the Student-$t$ distributions and the number of clusters in the simulated data.

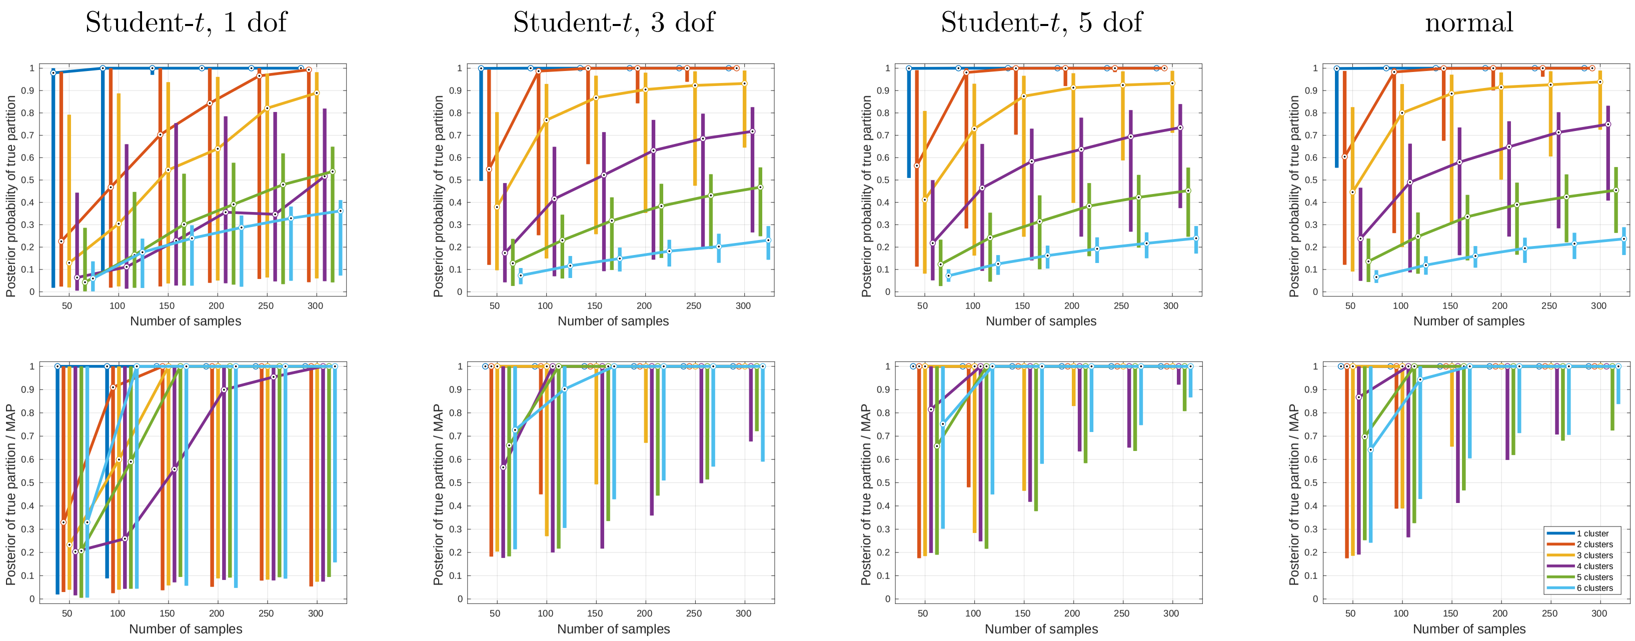


Figure 5: **Simulation study.** For `BayesOptim`, boxplot (median and $[25\%, 75\%]$ probability interval) of posterior probability for the true model (top) and ratio of posterior probability of true model to posterior probability of maximum a posteriori (bottom) for data of various types.

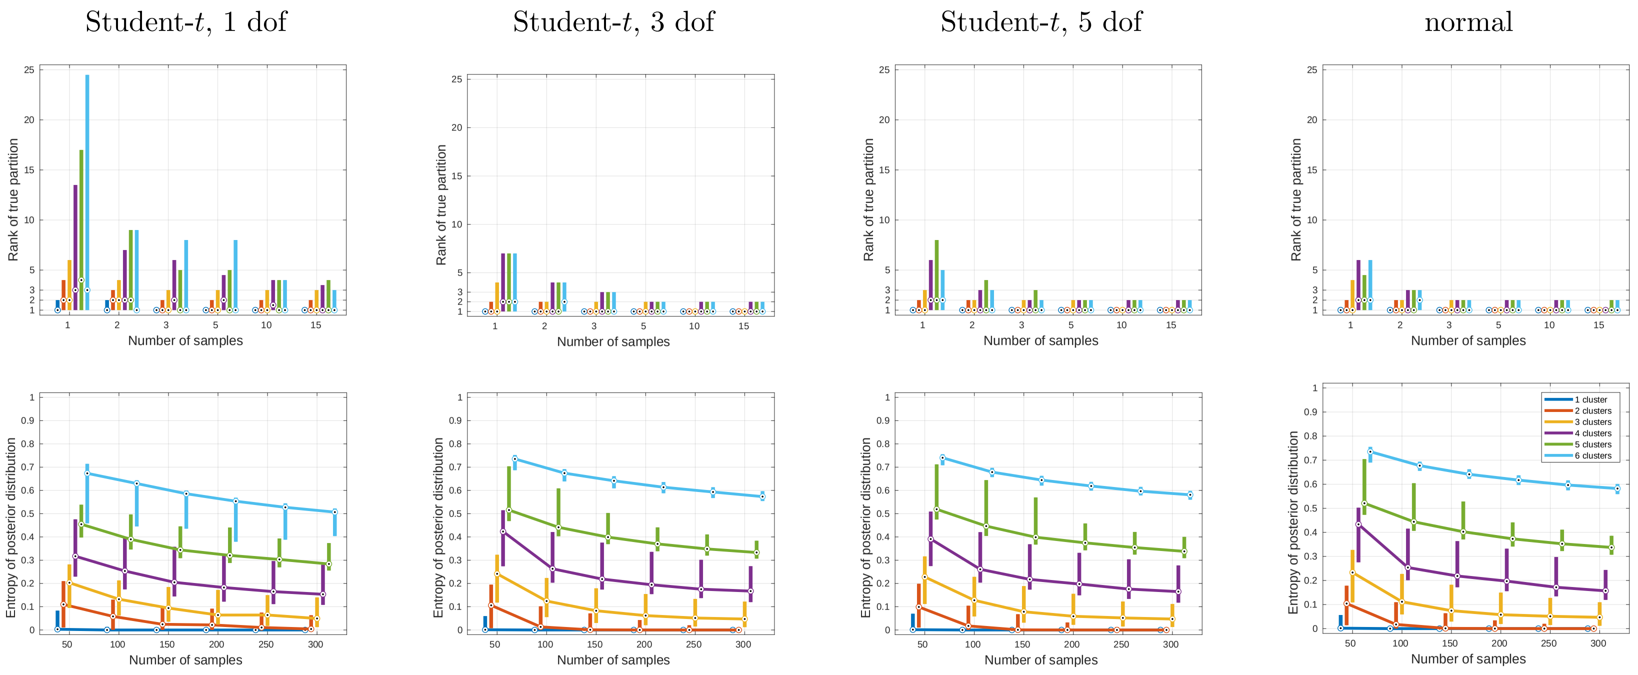


Figure 6: **Simulation study.** For `BayesOptim`, boxplot (median and $[25\%, 75\%]$ probability interval) of rank of true model when ranking potential models by decreasing posterior probability (top) and entropy of posterior distribution (bottom) for data of various types.

# 5 HIV study data

In Table 1, we reported the relevances [7] associated to the HIV study data.

Table 1: HIV study: Relevances from the exact probability distribution `BayesOptim`.

| Cardinality | Set | Relevance | Cardinality | Set | Relevance |
|---|---|---|---|---|---|
| | | | 6 | 123456 | $3.90 \times 10^{-5}$ |
| 1 | 1 | $1.40 \times 10^{-6}$ | 5 | 23456 | $1.57 \times 10^{-10}$ |
| | 2 | $2.40 \times 10^{-5}$ | | 13456 | $1.25 \times 10^{-8}$ |
| | 3 | $3.43 \times 10^{-7}$ | | 12456 | $1.68 \times 10^{-10}$ |
| | 4 | 0.994 | | 12356 | 0.852 |
| | 5 | $4.63 \times 10^{-9}$ | | 12346 | $4.89 \times 10^{-14}$ |
| | 6 | $1.80 \times 10^{-3}$ | | 12345 | $7.25 \times 10^{-7}$ |
| 2 | 12 | 0.134 | 4 | 3456 | $8.35 \times 10^{-4}$ |
| | 13 | $1.70 \times 10^{-13}$ | | 2456 | $1.44 \times 10^{-16}$ |
| | 14 | $1.49 \times 10^{-7}$ | | 2356 | $2.43 \times 10^{-7}$ |
| | 15 | $3.25 \times 10^{-13}$ | | 2346 | $1.15 \times 10^{-16}$ |
| | 16 | $5.93 \times 10^{-8}$ | | 2345 | $4.06 \times 10^{-11}$ |
| | 23 | $1.24 \times 10^{-13}$ | | 1456 | $5.42 \times 10^{-15}$ |
| | 24 | $7.46 \times 10^{-6}$ | | 1356 | $3.03 \times 10^{-5}$ |
| | 25 | $8.54 \times 10^{-15}$ | | 1346 | $2.35 \times 10^{-17}$ |
| | 26 | $2.90 \times 10^{-7}$ | | 1345 | $9.54 \times 10^{-10}$ |
| | 34 | $1.35 \times 10^{-7}$ | | 1256 | $4.54 \times 10^{-7}$ |
| | 35 | $9.21 \times 10^{-3}$ | | 1246 | $1.61 \times 10^{-5}$ |
| | 36 | $8.72 \times 10^{-9}$ | | 1245 | $1.71 \times 10^{-10}$ |
| | 45 | $2.30 \times 10^{-9}$ | | 1236 | $1.80 \times 10^{-10}$ |
| | 46 | $2.57 \times 10^{-4}$ | | 1235 | $1.01 \times 10^{-3}$ |
| | 56 | $6.41 \times 10^{-10}$ | | 1234 | $8.49 \times 10^{-13}$ |
| 3 | 123 | $1.69 \times 10^{-10}$ | | | |
| | 124 | $3.82 \times 10^{-3}$ | | | |
| | 125 | $2.60 \times 10^{-8}$ | | | |
| | 126 | $8.86 \times 10^{-3}$ | | | |
| | 134 | $4.52 \times 10^{-15}$ | | | |
| | 135 | $1.16 \times 10^{-7}$ | | | |
| | 136 | $1.09 \times 10^{-14}$ | | | |
| | 145 | $1.96 \times 10^{-14}$ | | | |
| | 146 | $5.37 \times 10^{-10}$ | | | |
| | 156 | $1.54 \times 10^{-12}$ | | | |
| | 234 | $1.16 \times 10^{-14}$ | | | |
| | 235 | $3.58 \times 10^{-9}$ | | | |
| | 236 | $1.91 \times 10^{-14}$ | | | |
| | 245 | $7.11 \times 10^{-16}$ | | | |
| | 246 | $6.78 \times 10^{-9}$ | | | |
| | 256 | $2.42 \times 10^{-14}$ | | | |
| | 345 | $7.23 \times 10^{-4}$ | | | |
| | 346 | $4.32 \times 10^{-10}$ | | | |
| | 356 | 0.136 | | | |
| | 456 | $2.69 \times 10^{-11}$ | | | |

# References

[1] T. W. Anderson, *An Introduction to Multivariate Statistical Analysis*, ser. Wiley Publications in Statistics. John Wiley and Sons, New York, 1958.

[2] A. Gelman, J. B. Carlin, H. S. Stern, and D. B. Rubin, *Bayesian Data Analysis*, ser. Texts in Statistical Science. Chapman & Hall, London, 1998.

[3] M. Abramowitz and I. A. Stegun, Eds., *Handbook of Mathematical Functions*, ser. Applied Math. National Bureau of Standards, 1972, no. 55.

[4] N. G. de Bruijn, *Asymptotic Methods in Analysis*, 2nd ed., ser. Bibliotheca Mathematica. A Series of Monographs on Pure and Applied Mathematics. North-Holland Publishing Co., Amsterdam, 1961, vol. IV.

[5] D. E. Knuth, *The Art of Computer Programming. Volume 4, Fascicle 3B*. Addison-Wesley, Boston, 2005.

[6] J. G. Booth, G. Casella, and J. P. Hobert, "Clustering using objective functions and stochastic search," *Journal of the Royal Statistical Society: Series B (Statistical Methodology)*, vol. 70, pp. 119–139, 2008.

[7] J. A. Hartigan, "Partition models," *Communications in Statistics. Theory and Methods*, vol. 19, pp. 2745–2756, 1990.
